# Supplementary material for: MBQ: Modality-Balanced Quantization for Large Vision-Language Models
Source: arXiv:2412.19509 source file (2025-03-21)
Supplement: Supplementary file 1 [file baseline.tex]

The image you've provided appears to be from the movie ``Titanic'', directed by James Cameron. The ending of the film is quite famous and involves a tragic event where the ship Titanic sinks after hitting an iceberg, leading to the deaths of many passengers, including the character Jack Dawson, played by Leonardo DiCaprio, who dies alongside the character Rose DeWittbrow, played by Kate Winslet. The scene depicted in the image shows Jack and Rose embracing as they prepare to go over the railing of the sinking ship, with Jack saying his famous line, ``I'm the king of the world.''
