# Supplementary material for: MBQ: Modality-Balanced Quantization for Large Vision-Language Models
Source: arXiv:2412.19509 source file (2025-03-21)
Supplement: Supplementary file 2 [file fp16.tex]

The image you've provided is from the movie ``Titanic'', directed by James Cameron. The ending of ``Titanic'' is quite well-known and involves a tragic event where the ship hits an iceberg and sinks, leading to the deaths of many passengers. The central characters, Jack Dawson and Rose DeWitt Bukater, are shown in the film's conclusion, with Jack sacrificing himself to save Rose by pushing her onto a piece of debris that allows her to stay afloat. Jack does not survive, and the film ends with Rose, now elderly, still wearing the diamond necklace Jack gave her, and looking out at the ocean, presumably remembering their story.
