# Supplementary material for: MBQ: Modality-Balanced Quantization for Large Vision-Language Models
Source: arXiv:2412.19509 source file (2025-03-21)
Supplement: Supplementary file 3 [file ours.tex]

The movie you're referring to is likely ``Titanic'', directed by James Cameron. The ending of this film is quite famous and involves a tragic event where the ship Titanic sinks after hitting an iceberg during its maiden voyage from Southampton to Cherbourg, France, on April 10, 1912. In the film's conclusion, the ship begins to list severely after taking on water in its starboard side compartments. Despite efforts by the crew to save passengers, the ship eventually breaks apart and sinks into the North Atlantic Ocean. The film portrays the tragic fate of the ship and its passengers, with a particular focus on the doomed romance between the characters Jack Dawson and Rose DeWittbuck. The film ends with Jack Dawson, who died in the disaster, being placed next to Rose on the stern of the sinking ship. The final scene shows the two characters embracing as the ship sinks beneath them, symbolizing their love that transcends even death itself.
