# Supplementary material for: MBQ: Modality-Balanced Quantization for Large Vision-Language Models
Source: arXiv:2412.19509 source file (2025-03-21)
Supplement: Supplementary file 5 [file baseline.tex]

这个梗可能是在描述这栋楼的外观设计，将其比喻为“中了二向箔一样”，这里的“二向箔”可能是指一种特殊的材料或者结构，但这个表述在日常语言中并不常见，所以具体含义可能需要根据上下文或当地方言来理解。通常，这种描述方式是在强调建筑的特殊性或不寻常的设计。
