# Supplementary material for: MBQ: Modality-Balanced Quantization for Large Vision-Language Models
Source: arXiv:2412.19509 source file (2025-03-21)
Supplement: Supplementary file 6 [file fp16.tex]

这个梗源自于刘慈欣的科幻小说《三体》。在小说中，二向箔是一种高科技武器，可以将三维空间压缩成二维，从而摧毁敌方的飞船或基地。当人们说“这栋楼就像中了二向箔一样”，通常是在形容一栋楼的外观设计非常独特，仿佛被某种力量压缩成了一个平面，失去了传统的三维立体感。这种描述方式带有一定的幽默感和夸张色彩，用来表达对现代建筑风格的惊奇和赞赏。
