# Supplementary material for: MBQ: Modality-Balanced Quantization for Large Vision-Language Models
Source: arXiv:2412.19509 source file (2025-03-21)
Supplement: Supplementary file 7 [file ours.tex]

这个梗源自于刘慈欣的科幻小说《三体》。在小说中，二向箔是一种高科技产品，可以将三维空间压缩成二维。当这栋楼被比喻为“中了二向箔”，意味着它在视觉上看起来像是被压缩成了二维，即变得非常薄。这种描述通常用于幽默地表达建筑物在某些角度下显得异常狭窄或扁平的外观。
