# Supplementary material for: MBQ: Modality-Balanced Quantization for Large Vision-Language Models
Source: arXiv:2412.19509 source file (2025-03-21)
Supplement: Supplementary file 8 [file question.tex]

“这栋楼就像中了二向箔一样”这个梗怎么理解
