# Supplementary material for: MBQ: Modality-Balanced Quantization for Large Vision-Language Models
Source: arXiv:2412.19509 source file (2025-03-21)
Supplement: Supplementary file 9 [file baseline.tex]

The humor in this meme comes from the juxtaposition of the text above and below the image. The top line sets up an expectation that the speaker's mother will find something funny, while the bottom line subverts that expectation by having the mother not understand or find humor in the same thing. It plays on the common experience where people share memes with their parents, only to realize they don't find them amusing.
