# Supplementary material for: MBQ: Modality-Balanced Quantization for Large Vision-Language Models
Source: arXiv:2412.19509 source file (2025-03-21)
Supplement: Supplementary file 10 [file fp16.tex]

The humor in this meme comes from the juxtaposition of a child's expectation that their parent will find something funny, with the reality that the parent doesn't understand or appreciate the humor. The image of Winnie the Pooh looking puzzled while reading a piece of paper symbolizes the confusion and lack of understanding that the parent feels when faced with what is supposed to be a funny meme.
