# Supplementary material for: MBQ: Modality-Balanced Quantization for Large Vision-Language Models
Source: arXiv:2412.19509 source file (2025-03-21)
Supplement: Supplementary file 11 [file ours.tex]

The humor in this meme comes from the juxtaposition of showing a funny meme to one's mom and her not finding it amusing. It plays on the stereotype that parents often don't understand or relate to the same things their children find funny, especially when it comes to internet culture.
