# Supplementary material for: MBQ: Modality-Balanced Quantization for Large Vision-Language Models
Source: arXiv:2412.19509 source file (2025-03-21)
Supplement: Supplementary file 12 [file question.tex]

Can you explain the humor in this meme featuring Winnie the Pooh?
